# Supplementary material for: Evolving Domain Adaptation of Pretrained Language Models for Text Classification
Source: arXiv:2311.09661 source file (2023-11-16)
Supplement: Supplementary file 1 [file domain_divergence.tex]

\section{Detailed Domain Divergence Analysis}
\label{sec:appendix-domain-divergence}

To better understand the performance trends observed in \Scref{sec:result_over_domain}, visualize the divergence between all pairs of domains, quantified by the MMD~\cite{gretton2012kernel} between their embeddings. 
% To quantify these shifts, we use Maximum Mean Discrepancy (MMD) \cite{gretton2012kernel}
% % \yw{Should we add citation for MMD} 
% with a Radial Basis Function (RBF) kernel to measure the distance between two distributions, computed based on the marginal distribution of text embeddings $P_{g(\Xcal)}$ projected by E5-Large-V2 model. 
% \paragraph{Analysis of Evolving Domain Shift}
% To better understand the performance trends observed in \Scref{sec:result_over_domain}, we delve into a deeper analysis of the evolving domain shifts. In this analysis, we particularly focus on the covariate shifts, changes in the distribution of input data, as reflected in the text embeddings. To quantify these shifts, we use Maximum Mean Discrepancy (MMD) \cite{gretton2012kernel}
% % \yw{Should we add citation for MMD} 
% with a Radial Basis Function (RBF) kernel to measure the distance between two distributions, computed based on the marginal distribution of text embeddings $P_{g(\Xcal)}$ projected by E5-Large-V2 model. The larger the MMD value, the more substantial the domain shift is. 
% MMD citation: Arthur Gretton, Karsten M Borgwardt, Malte J Rasch, Bernhard Schölkopf, and Alexander Smola. A kernel two-sample test. Journal of Machine Learning Research, 13(Mar):723–773, 2012.
Critically, for both datasets, the MMD between two adjacent domains is almost always smaller than the MMD between the source and any target domain. This observation supports our earlier findings on the advantage of maintaining a dynamic buffer over relying on static source domain data for adapting to evolving domains.

% Significantly, the MMD between each pair of adjacent domains is almost always smaller than the MMD between the source domain and any given target domain. This observation supports our earlier findings on the advantage of maintaining a dynamic buffer over relying on static source domain data for adapting to evolving domains.
\paragraph{COVID Dataset}
Figure~\ref{fig:mat_dist_mmd_covid_marginal} showcases the domain shift over the marginal distribution of each domain. The domain shift is more gradual and uni-directional. The MMD between the source domain and the subsequent target domains increases over time, aligning with the gradual decay observed in the \tunesource baseline in Figure~\ref{fig:tuning_gda_covid}. This indicates a gradual evolution of the COVID discussion space over time, with newer content becoming progressively more distinct from the initial discussions.
We see very similar structure when analysing the divergence between label conditional distributions for each domain. Figures~\ref{fig:mat_dist_mmd_covid_against} and~\ref{fig:mat_dist_mmd_covid_not_against} showcase the pairwise MMD between the conditional distributions for the ``Against'' and ``Not-Against'' classes respectively.

% For both datasets, Figures 
% Figure~\ref{fig:mat_dist_mmd_covid_against} and~\ref{fig:mat_dist_mmd_covid_not_against} is the MMD on COVID with label Against and Not-against, respectively. 

\paragraph{WTWT}
In contrast, the domain shift in the WTWT dataset (Figure~\ref{fig:mat_dist_mmd_wtwt_marginal}) is more abrupt, with notable discontinuities. Two most substantial discontinuities occur around the 17-07 domain and another around the 18-05 domain, in line with the abrupt shift in topic distribution as shown in Table~\ref{tab:topic_dist_over_time_wtwt}. Notably, we observe an inverted-U shape trend when using the source domain as an anchor point: the MMD between the source domain and any given target domain peaks around 17-07 and subsequently declines. This pattern is consistent with the changes in the topic distribution, especially the rise and fall of the FOXA v.s. DIS topic around this period. As the FOXA v.s. DIS topic, related to events in the entertainment sector, is significantly different from the other four topics, all in the pharmaceutical sector, it contributes to the inverted-U shape in domain shift. This also aligns with the performance trend of the \tunesource baseline model in Figure~\ref{fig:tuning_gda_wtwt}. 
% \ru{I can't find the figure, could you add the correct reference @Sean?}

\begin{figure}[htbp!] % use figure for single-column figures
\centering
\includegraphics[width=\linewidth]{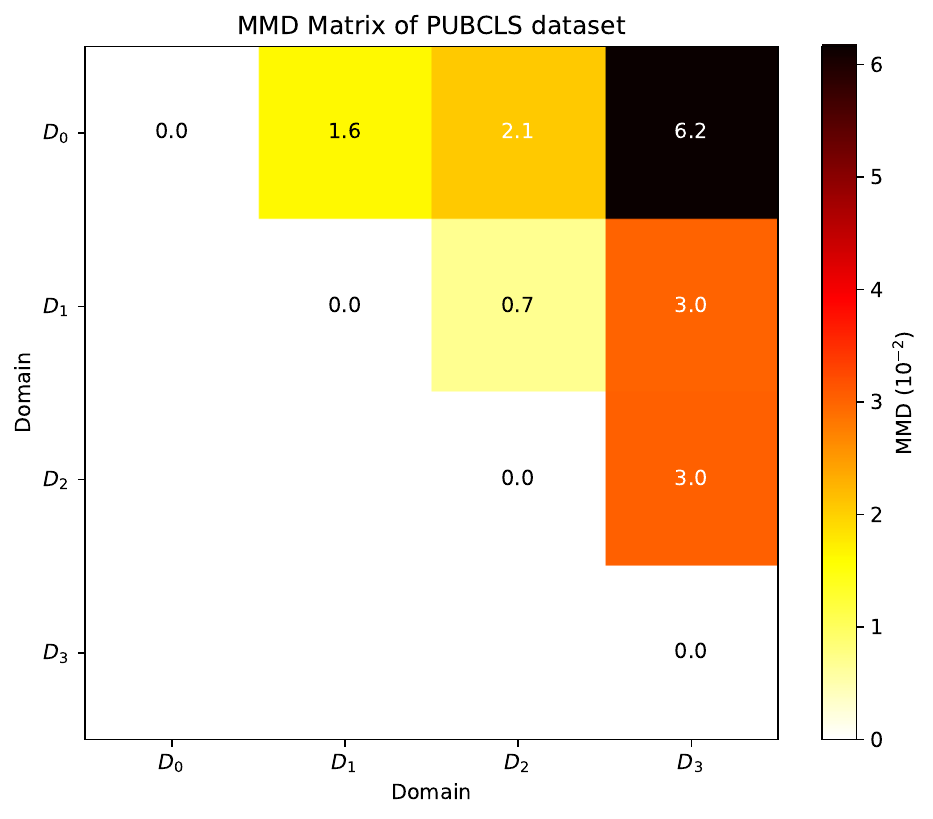}
\caption{Maximum Mean Discrepancy (MMD) matrix of the SciERC Dataset. Each cell represents the MMD between a pair of domains, calculated based on the marginal distribution of text embeddings $P_{g(\Xcal)}$ projected by the E5-Large-V2 model. The color gradient ranges from white (representing zero discrepancy) to darker shades of red (indicating larger discrepancies). Please note that the numbers in the heatmap are in the units of $10^{-2}$.}
\label{fig:mat_dist_mmd_sci_erc_marginal}
\end{figure}

\begin{figure}[htbp!] % use figure for single-column figures
\centering
\includegraphics[width=\linewidth]{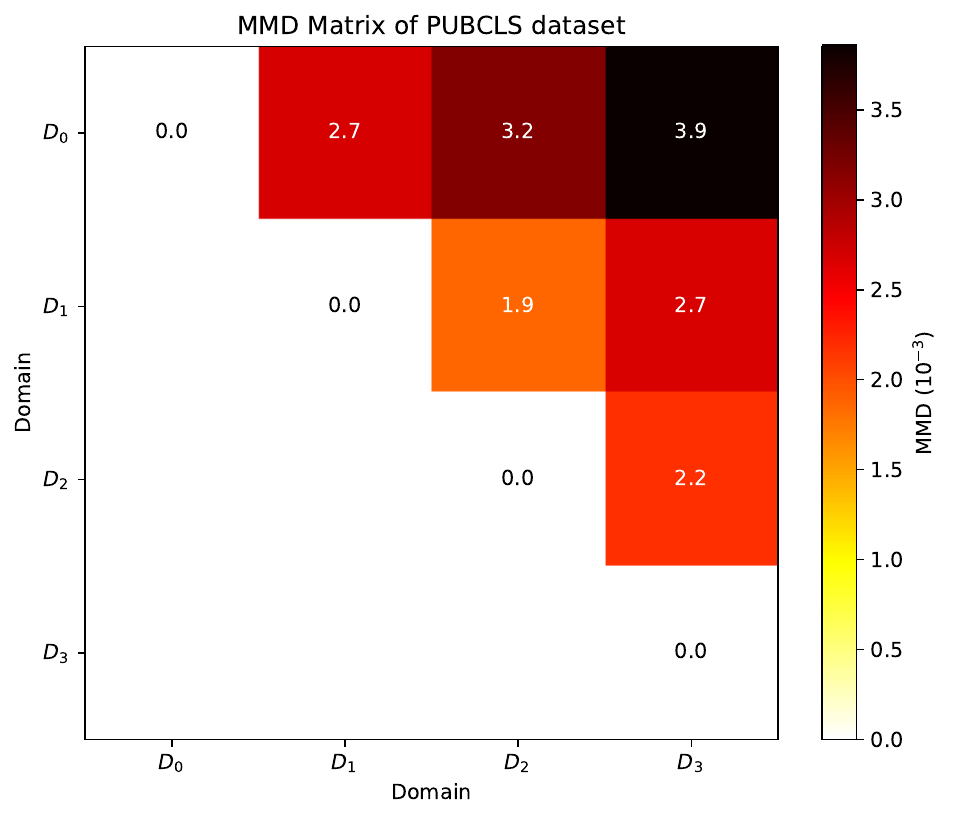}
\caption{Maximum Mean Discrepancy (MMD) matrix of the PUBCLS Dataset. Each cell represents the MMD between a pair of domains, calculated based on the marginal distribution of text embeddings $P_{g(\Xcal)}$ projected by the E5-Large-V2 model. The color gradient ranges from white (representing zero discrepancy) to darker shades of red (indicating larger discrepancies). Please note that the numbers in the heatmap are in the units of $10^{-2}$.}
\label{fig:mat_dist_mmd_pubcls_marginal}
\end{figure}
