# Supplementary material for: Evolving Domain Adaptation of Pretrained Language Models for Text Classification
Source: arXiv:2311.09661 source file (2023-11-16)
Supplement: Supplementary file 2 [file oic_details.tex]

\section{Detailed Formula of \onlineexp}
\label{sec:appendix-online-prompt}
For clarification, we formally define some seemingly obvious formulas about \onlineexp (\Scref{sec:method-example-selection}).

% \subsection{Computing Mean Embedding $\mu_{t-1}^y$}
% \label{sec:appendix-online-prompt-mean-emb}
% In Equation \ref{eq:find_mean_emb_1}, $h$ is a function that finds the mean embedding within buffer $B$ that belongs to class $y$. $h$ is formally defined as:

% \begin{align}
% \label{eq:find_mean_emb_2}
% h(\Bcal, y) = \frac{1}{\sum_{(x_i, y_i) \in \Bcal} \mathbbm{1}_{y_i = y}} \sum_{\substack{(x_i, y_i) \in \Bcal,\ y_i = y}} g(x_i),
% \end{align}

% where $\sum_{(x_i, y_i) \in \Bcal} \mathbbm{1}_{y_i = y}$ is the count of instances of class $y$ in the buffer $\Bcal$, and $g:\Xcal \to \mathbb{R}^d$ is a pre-trained language model encoder.

\subsection{Finding the Most Representative Example}
\label{sec:appendix-online-prompt-find-rep}
When constructing the in-context examples in Eq.~(\ref{eq:make_C}), we
use the most representative example for class $y$ as the example whose embedding is closest to the mean embedding $\ub_{t-1}^y$. Formally, the representative example for class $y$ at time $t-1$, denoted as $(x_\text{rep}, y)$, is selected as follows:

\begin{align}
(x_\text{rep}, y) = \argmax_{(x_i, y_i) \in \Bcal_{t-1}, y_i = y} \cos(g(x_i), \ub_{t-1}^y),
\end{align}
where $\cos(g(x_i), \ub_{t-1}^y)$ is the cosine similarity between the embedding of example $x_i$ and the mean embedding $\ub_{t-1}^y$ for class $y$. This would select the example whose embedding $g(x)$ is the most similar to the mean embedding of class $y$.
