# Supplementary material for: Evolving Domain Adaptation of Pretrained Language Models for Text Classification
Source: arXiv:2311.09661 source file (2023-11-16)
Supplement: Supplementary file 3 [file f1_ratio_baseline_over_supervised.tex]

\begin{table*}[htbp!]
\centering
\small
    \begin{tabular}{lllll}
    \toprule
    Domain Type & Domain & baseline & supervised & Ratio \\
    \midrule
    Source Domain & $\Dcal_0$: 2020-12 to 2021-05 & 0.654 & 0.748 & 0.874 \\
    \cmidrule{2-5}
    Target Domains & $\Dcal_1$: 2021-06 & 0.569 & 0.638 & 0.892 \\
    & $\Dcal_2$: 2021-07 & 0.566 & 0.658 & 0.861 \\
    & $\Dcal_3$: 2021-08 & 0.629 & 0.727 & 0.865 \\
    & $\Dcal_4$: 2021-09 & 0.534 & 0.696 & 0.768 \\
    & $\Dcal_5$: 2021-10 & 0.409 & 0.691 & 0.593 \\
    & $\Dcal_6$: 2021-11 & 0.516 & 0.721 & 0.716 \\
    & $\Dcal_7$: 2021-12 & 0.470 & 0.703 & 0.668 \\
    & $\Dcal_8$: 2022-01 & 0.444 & 0.626 & 0.709 \\
    & $\Dcal_9$: 2022-02 to 2022-03 & 0.462 & 0.680 & 0.679 \\
    & $\Dcal_{10}$: 2022-04 to 2022-06 & 0.491 & 0.732 & 0.671 \\
    \bottomrule
    \end{tabular}
\caption{Ratios of F1-macro scores between gda\_baseline and supervised methods in COVID dataset}
\label{tab:ratio_f1_macro_between_baseline_supervised_covid}
\end{table*}

\begin{table*}[htbp!]
  \centering
  \small
  {
    \begin{tabular}{lllll}
    \toprule
    Domain Type & Domain & baseline & supervised  & Ratio \\
    \midrule
    Source Domain & $\Dcal_0$: 2015-06 to 2016-06 & 0.783 & 0.802 & 0.976 \\
    \cmidrule{2-5}
    Target Domains & $\Dcal_1$: 2016-07 to 2016-08 & 0.783 & 0.788 & 0.993 \\
    & $\Dcal_2$: 2016-09 to 2016-10 & 0.788 & 0.811 & 0.972 \\
    & $\Dcal_3$: 2016-11 to 2016-12 & 0.779 & 0.806 & 0.967 \\
    & $\Dcal_4$: 2017-01 to 2017-02 & 0.727 & 0.776 & 0.937 \\
    & $\Dcal_5$: 2017-03 to 2017-06 & 0.682 & 0.764 & 0.893 \\
    & $\Dcal_6$: 2017-07 to 2017-08 & 0.383 & 0.806 & 0.476 \\
    & $\Dcal_7$: 2017-09 to 2017-10 & 0.464 & 0.819 & 0.566 \\
    & $\Dcal_8$: 2017-11 to 2017-12 & 0.432 & 0.786 & 0.550 \\
    & $\Dcal_9$: 2018-01 to 2018-02 & 0.476 & 0.784 & 0.607 \\
    & $\Dcal_{10}$: 2018-03 to 2018-04 & 0.519 & 0.781 & 0.665 \\
    & $\Dcal_{11}$: 2018-05 to 2018-06 & 0.681 & 0.743 & 0.916 \\
    & $\Dcal_{12}$: 2018-07 to 2018-08 & 0.646 & 0.758 & 0.853 \\
    & $\Dcal_{13}$: 2018-09 to 2018-10 & 0.655 & 0.749 & 0.875 \\
    & $\Dcal_{14}$: 2018-11 to 2018-12 & 0.640 & 0.817 & 0.784 \\
    \bottomrule
    \end{tabular}
}
\caption{Ratios of F1-macro scores between gda\_baseline and supervised methods in WTWT dataset}
  \label{tab:ratio_f1_macro_between_baseline_supervised_wtwt}
\end{table*}

\begin{table*}[htbp!]
  \centering
  \small
  {
    \begin{tabular}{lllll}
    \toprule
    Domain Type & Domain & baseline & supervised & Ratio \\
    \midrule
    Source Domain & $\Dcal_0$: 2009 to 2010 & 0.527 & 0.771 & 0.684 \\
    \cmidrule{2-5}
    Target Domains & $\Dcal_1$: 2011 to 2012 & 0.485 & 0.826 & 0.587 \\
    & $\Dcal_2$: 2013 to 2014 & 0.490 & 0.848 & 0.578 \\
    & $\Dcal_3$: 2015 to 2016 & 0.480 & 0.791 & 0.606 \\
    \bottomrule
    \end{tabular}

}
\caption{Ratios of F1-macro scores between gda\_baseline and supervised methods in PUBCLS dataset}
  \label{tab:ratio_f1_macro_between_baseline_supervised_pubcls}
\end{table*}

\begin{table*}[htbp!]
  \centering
  \small
  {
        \begin{tabular}{lllll}
        \toprule
        Domain Type & Domain & baseline & supervised & Ratio \\
        \midrule
        Source Domain & $\Dcal_0$: 1980 to 1999 & 0.713 & 0.729 & 0.978 \\
        \cmidrule{2-5}
        Target Domains & $\Dcal_1$: 2000 to 2004 & 0.518 & 0.667 & 0.778 \\
        & $\Dcal_2$: 2005 to 2009 & 0.421 & 0.630 & 0.668 \\
        & $\Dcal_3$: 2010 to 2016 & 0.280 & 0.658 & 0.425 \\
        \bottomrule
        \end{tabular}
        
        }
\caption{Ratios of F1-macro scores between gda\_baseline and supervised methods in SCI\_ERC dataset}
  \label{tab:ratio_f1_macro_between_baseline_supervised_sci_erc}
\end{table*}
