# Supplementary material for: Evolving Domain Adaptation of Pretrained Language Models for Text Classification
Source: arXiv:2311.09661 source file (2023-11-16)
Supplement: Supplementary file 4 [file norm_score_tables.tex]

\label{sec:norm_score_tables}

% \begin{table}[tbp!]
%   \centering  
%   % \small
%    \resizebox{\linewidth}{!}{  
%   \begin{tabular}{llllll}
%     \toprule
%     Methods & Variants & \multicolumn{4}{c}{Dataset} \\ 
%     \cmidrule{3-6}
%     & & COVID & WTWT & SCIERC & PUBCLS \\
%     \midrule
%     Baseline & \tunesource & 0.509 & 0.618 & 0.485 & 0.406 \\
%     \midrule       
%     Self-training & \offline & 0.460 (-28) & 0.633 (9) & 0.593 (32) & 0.363 (-18)\\    
%      & \onlinebuf  & 0.569 (34) & 0.697 (47) & 0.520 (10) & 0.469 (26) \\
%      & \onlinecum  & \textbf{0.611 (57)} & \textbf{0.739 (72)} & \textbf{0.684 (59)} & \textbf{0.492 (35)} \\
%     % \midrule       
%     DANN & - & 0.519 (6) & 0.647 (17) & 0.511 (8) & 0.440 (14)\\
%     DAPT & - & 0.524 (8) & 0.664 (28) & 0.503 (5) & 0.458 (21)\\
%     \midrule    
%     \tunetrue & - & 0.687 & 0.785 & 0.822 & 0.651 \\    
%     \bottomrule
%   \end{tabular}
%   }
%   \caption{Normalized Performance metrics ($F_\text{avg}$) across methods for the BERT-large model on all datasets.}
%   \label{tab:performance_metrics_tuning}
%   \vspace{-3mm}
% \end{table}

\begin{table}[tbp!]
  \centering  
  \small
   \resizebox{\linewidth}{!}{  
      \begin{tabular}{lllll}
        \toprule
        Methods & Variants & \multicolumn{3}{c}{Dataset} \\ % change moulti column from {4}{c} to {3}{c}
        \cmidrule{3-5} % change from {3-6} to {3-5}
        & & COVID & SCIERC & PUBCLS \\
        \midrule    
        \promptzero & - & 0.772  &  0.348 & -\\
        \midrule
        Baseline & \tunesource & 0.795  &  0.809 & -\\
        \midrule       
        Self-training & \offline & 0.816 (46)  &  0.820 (22) & -\\    
         & \onlinebuf  & 0.812 (37)  &  0.822 (39) & - \\    
         & \onlinecum  & \textbf{0.821 (57)}  & \textbf{0.842 (100)} & -\\
        % \midrule       
        DAPT & - & 0.731 & 0.503 & 0.458  \\   %WTWT was 0.664
        \midrule    
        \tunetrue & - & 0.841 & 0.842 & - \\    % WTWT was ? before
        \bottomrule
      \end{tabular}
  }
  \caption{Normalized Performance metrics ($F_\text{avg}$) across methods for the FLAN-T5-XXL model on all datasets except WTWT. \sn{Should also mention the Zero baseline}}
  \label{tab:performance_metrics_tuning}
  \vspace{-5mm}
\end{table}
